# Supplementary material for: Deep Concept-wise Temporal Convolutional Networks for Action Localization
Source: arXiv:1908.09442 source file (2019-08-26)
Supplement: Supplementary file 1 [file CTCN_SM.pdf]

# Deep Concept-wise Temporal Convolutional Networks for Action Localization (Supplementary Material)

Xin Li[1], Tianwei Lin[1], Xiao Liu[1], Chuang Gan[2], Wangmeng Zuo[3], Chao Li[1],
Xiang Long[1], Dongliang He[1], Fu Li[1], Shilei Wen[1]
Department of Computer Vision Technology (VIS), Baidu Inc.[1]
MIT-Watson AI Lab.[2] Harbin Institute of Technology.[3]

## A. Content

The content of this supplementary material involves:

- The architecture of C-TCN.
- Additional results about how group convolution and weight sharing contribute to the performance improvement of C-TCN.

## B. Architecture Details

Our C-TCN is comprised of three components, *i.e.*, the backbone, the feature pyramid and the predictor head.

The backbone architecture of C-TCN is shown in Table A. The shape of an input sample is $1 \times 256 \times 512$. We use two CTC layers with stride to make $C_1$, who is then passed to a ResNet with 4 stages of CTC residual blocks to produce $C_2$ to $C_5$. Batch normalization and ReLU are added to the end of each CTC layer.

The feature pyramid architecture of C-TCN is shown in Table B. $P_6$ is computed via a $1 \times 3$ CTC layer with $1 \times 2$ stride on $C_5$. $P_7$ to $P_9$ are obtained by applying ReLU followed by a $1 \times 3$ CTC layer with $1 \times 2$ stride on the previous scale correspondingly. We then compute $P_2$ to $P_5$ based on $C_2$ to $C_5$ using top-down and lateral connections.

Table A: The backbone architecture of C-TCN. The shape of an input sample is $1 \times 256 \times 512$. We use two CTC layers with stride to make $C_1$, who is then passed to a ResNet with 4 stages of CTC residual blocks to produce $C_2$ to $C_5$. Batch normalization and ReLU are added to the end of each CTC layer.

| backbone stage | output | architecture |
|---|---|---|
| $C_1$ | $64 \times 256 \times 128$ | $1 \times 7$ conv, stride $1 \times 2$, 32<br>$1 \times 7$ conv, stride $1 \times 2$, 64 |
| $C_2$ | $256 \times 256 \times 128$ | $\begin{bmatrix} 1 \times 1 & \text{conv}, 128 \\ 1 \times 3 & \text{conv}, 128 \\ 1 \times 1 & \text{conv}, 512 \end{bmatrix} \times 3$ |
| $C_3$ | $512 \times 256 \times 64$ | $\begin{bmatrix} 1 \times 1 & \text{conv}, 256 \\ 1 \times 3 & \text{conv}, 256 \\ 1 \times 1 & \text{conv}, 1024 \end{bmatrix} \times 4$ |
| $C_4$ | $1024 \times 256 \times 32$ | $\begin{bmatrix} 1 \times 1 & \text{conv}, 512 \\ 1 \times 3 & \text{conv}, 512 \\ 1 \times 1 & \text{conv}, 2048 \end{bmatrix} \times 6$ |
| $C_5$ | $2048 \times 256 \times 16$ | $\begin{bmatrix} 1 \times 1 & \text{conv}, 1024 \\ 1 \times 3 & \text{conv}, 1024 \\ 1 \times 1 & \text{conv}, 4096 \end{bmatrix} \times 3$ |

The predictor head architecture of C-TCN is shown in Table C. We use two predictor heads for temporal segment classifier and regressor separately. Each predictor head has a hidden layer followed by a prediction layer. The hidden layer is a $1 \times 3$ CTC layer that decreases the potential number to 256. The prediction layer is a $256 \times 1$ convolutional layer that combines information from all concepts. It produces a $(A+1)M$-channel $2^{9-l}$-length score map for $P_l$, where $A+1$ is the number of action categories plus one background class, $l$ is the pyramid scale and $M$ is the number of anchor segments. Hence, the temporal segment classifier produces classification scores for $M$ anchor segments at each temporal location and scale of pyramid. Similarly, the prediction layer of the regressor produces a $2M$-channel $2^{9-l}$-length output for $P_l$. The location and size offsets are predicted for each anchor segment at each temporal location and scale of pyramid.

Table B: The feature pyramid architecture of C-TCN. $P_6$ is computed via a $1 \times 3$ CTC layer with $1 \times 2$ stride on $C_5$. $P_7$ to $P_9$ are obtained by applying ReLU followed by a $1 \times 3$ CTC layer with $1 \times 2$ stride on the previous scale correspondingly. We then compute $P_2$ to $P_5$ based on $C_2$ to $C_5$ using top-down and lateral connections.

| feature pyramid | output | architecture |
|---|---|---|
| $P_2$ | $512 \times 256 \times 128$ | $1 \times 1$ conv, 512 ($C_2$)<br>upsample ($P_3$)<br>element-wise add<br>$1 \times 3$ conv, 512 |
| $P_3$ | $512 \times 256 \times 64$ | $1 \times 1$ conv, 512 ($C_3$)<br>upsample ($P_4$)<br>element-wise add<br>$1 \times 3$ conv, 512 |
| $P_4$ | $512 \times 256 \times 32$ | $1 \times 1$ conv, 512 ($C_4$)<br>upsample ($P_5$)<br>element-wise add<br>$1 \times 3$ conv, 512 |
| $P_5$ | $512 \times 256 \times 16$ | $1 \times 1$ conv, 512 ($C_5$) |
| $P_6$ | $512 \times 256 \times 8$ | $1 \times 3$ conv, stride $1 \times 2$, 512 ($C_5$) |
| $P_7$ | $512 \times 256 \times 4$ | $1 \times 3$ conv, stride $1 \times 2$, 512 ($P_6$) |
| $P_8$ | $512 \times 256 \times 2$ | $1 \times 3$ conv, stride $1 \times 2$, 512 ($P_7$) |
| $P_9$ | $512 \times 256 \times 1$ | $1 \times 3$ conv, stride $1 \times 2$, 512 ($P_8$) |

Table C: The predictor head architecture of C-TCN. We use two predictor heads for temporal segment classifier and regressor separately. Each predictor head has a hidden layer followed by a prediction layer. The hidden layer is a $1 \times 3$ CTC layer that decreases the potential number to 256. The prediction layer is a $256 \times 1$ convolutional layer that combines information from all concepts. It produces a $(A+1)M$-channel $2^{9-l}$-length score map for $P_l$, where $A+1$ is the number of action categories plus one background class, $l$ is the pyramid scale and $M$ is the number of anchor segments. Hence, the temporal segment classifier produces classification scores for $M$ anchor segments at each temporal location and scale of pyramid. Similarly, the prediction layer of the regressor produces a $2M$-channel $2^{9-l}$-length output for $P_l$.

| predictor head | output | architecture |
|---|---|---|
| classifier of $P_l$ | $256 \times 256 \times 2^{9-l}$<br>$(A+1)M \times 1 \times 2^{9-l}$<br>$(A+1)M \times 2^{9-l}$ | $1 \times 3$ conv, 256<br>$256 \times 1$ conv, $(A+1)M$<br>squeeze |
| regressor of $P_l$ | $256 \times 256 \times 2^{9-l}$<br>$2M \times 1 \times 2^{9-l}$<br>$2M \times 2^{9-l}$ | $1 \times 3$ conv, 256<br>$256 \times 1$ conv, $2M$<br>squeeze |

Table D: Ablation study on how group convolution and weight sharing contribute to the performance improvement of C-TCN. The results in terms of mAP(%) on the testing set of THUMOS'14 are reported.

| | without weight sharing | | | | | with weight sharing | | | | |
|---|---|---|---|---|---|---|---|---|---|---|
| tIoU | 0.1 | 0.2 | 0.3 | 0.4 | 0.5 | 0.1 | 0.2 | 0.3 | 0.4 | 0.5 |
| 1 group | 56.4 | 53.8 | 50.4 | 43.8 | 36.3 | 56.4 | 53.8 | 50.4 | 43.8 | 36.3 |
| 4 groups | 57.9 | 55.5 | 51.8 | 46.0 | 36.0 | 58.6 | 57.2 | 52.8 | 46.2 | 38.2 |
| 16 groups | 59.6 | 57.2 | 52.7 | 46.1 | 36.8 | 62.3 | 60.7 | 56.9 | 50.4 | 40.9 |
| 64 groups | 62.6 | 59.8 | 55.2 | 47.9 | 36.1 | 66.6 | 65.2 | 61.8 | 53.6 | 43.1 |
| 256 groups | 39.5 | 36.4 | 31.5 | 24.8 | 18.1 | 72.2 | 71.4 | 68.0 | 62.3 | 52.1 |

## C. Experiments on Group Convolution and Weight-Sharing

We conduct an additional experiment on THUMOS'14 to investigate how group convolution and weight sharing contribute to the performance improvement of C-TCN. The left part of Table D summarizes the results of five TCNs (60 layers) with different number of group convolutions. The right part of Table D summarizes the results of five TCNs with different number of group convolutions, but the filter parameters are shared by all groups. All models are optimally tuned on the validation set of THUMOS'14 and tested on the testing set. We see that: 1) solely using group convolution to avoid concept recombination is not enough for boosting the performance, because more groups cannot bring performance gain. 2) Using the same number of group, weight-sharing consistently improves the performance. 3) With weight-sharing, the performance can be consistently improved by increasing group numbers. Note that when the group number of TCN is 1 and parameters are not shared, it defines a standard TCN. And when the group number of TCN is 256 and the parameters are shared, it equals to a C-TCN. Thus, both group convolution and weight sharing in C-TCN are necessary for boosting the performance of temporal action localization.
